# Supplementary material for: Measuring algorithmic interpretability: A human-learning-based framework and the corresponding cognitive complexity score
Source: arXiv:2205.10207 source file (2022-05-20)
Supplement: Supplementary file 1 [file appendix.tex]

%appendix
\begin{comment}
\section{Ethical considerations}
As this work touches on concepts from the FATE community, we briefly discuss the potential ethical considerations of this work below.

One risk with the proposed framework is that quantifying interpretability devolves into just another metric to optimize.
Firms or developers may try to ``optimize'' interpretability by cutting corners on algorithms or obfuscating steps to reduce the interpretability score.
Such behaviors diminish the expected benefits of measuring interpretability, and should be avoided.
In particular, such attempts to game interpretability will involve introducing operations that certain users have not acquired as schemas, making the algorithm less interpretable.
That said, such risks are present for any such measurement, and safeguards that currently exist can also be applied here.
Peer-review of interpretability metrics as a regular part of new algorithm development will ensure that claims made about the interpretability of an algorithm are validated.
Regulatory bodies can check reported interpretability metrics via audits.

\section{Theoretical Analysis}
Here we pull together the structured programming theorem, the abstraction principle, and cognitive load theory to prove the following theorem:


\todo{link operations and schemas, selection and iteration with context}


\begin{theorem}[T1]
	Any algorithm can be represented as an~\graphname~graph.
\end{theorem} 

For this proof we need the following definitions:

\begin{definition}{}
	A \textit{schema} is an internalized sequence of operations that can be represented as a function representing an abstracted code block, or an operation node representing an abstracted subgraph.
\end{definition} 

\begin{definition}{}
	
\end{definition}


\begin{proof}{Proof} 
	We know from the structured program theorem that any computable algorithm can be represented as a control flow graph of sequences, selections, and iterations.
	Let's assume that some algorithm has been implemented in code as a fully abstracted object (i.e.,, a single function call runs the algorithm).
	This object can then be converted to an (optional) input node, the algorithm node, and an (optional) output node as a sequential control flow graph. 
	This \graphname~graph is not useful to most.
	In fact such \graphname~graphs may only be useful to the individual that wrote the code.
	However, the code or the graph can be decomposed based on a predefined set of schema.
	This decomposition is the same algorithm, and can therefore also be converted to an \graphname~graph.\Halmos
\end{proof}

One benefit of this result is that it can be operationalized in two ways. 
First, one may decompose abstractions in the code, by replacing abstracted methods with the lines of code that the method runs.
Then, once the appropriate level has been reached, this new program can be converted into a control flow graph and then an~\graphname.
On the other hand, one can convert the fully abstracted function to a graph, then do the decomposition on the graph until the appropriate~\graphname~is found.
The two will provide equivalent results.

\begin{corollary}{}
	For a given task, a more complex algorithm with have a wider range of interpretability scores.
\end{corollary} 

\begin{proof}{Proof}
	More complex algorithm means more complex operations, which will require further decomposition than a simpler algorithm. \Halmos
\end{proof}

\begin{theorem}[T2]
    \scorename is inversely proportional to the cyclomatic complexity of \cite{mccabeComplexityMeasure1976}. Structured programs can be reduced to graphs where cyclomatic complexity is one (as in Figure 1a). 
\end{theorem}

\todo{some details here around why this is true.} 


\subsection{Human-machine tradeoff}

Higher \scorename~implies more ``machine readable'' code.
This is due to the fact that as \scorename~decreases, it moves to a higher level of abstraction (i.e., more code ``behind the scenes'').
Graphs with a higher \scorename~consist of simpler operations, and at the upper bound consist of only addition, subtraction, multiplication, and division operatios (plus the associated contexts).
While this graph is certainly complex and not easy to read, it is \textit{simple} from an operations point of view.
\end{comment}
